# Supplementary material for: FedAttack: Effective and Covert Poisoning Attack on Federated Recommendation via Hard Sampling
Source: arXiv:2202.04975 source file (2022-02-10)
Supplement: Supplementary file 1 [file supplement.tex]

\section{Supplementary Materials}
